# Supplementary material for: Privacy and Integrity Preserving Training Using Trusted Hardware
Source: arXiv:2105.00334 source file (2021-05-01)
Supplement: Supplementary file 1 [file Appendix4.tex]

\section{Integrity}
As explained in section \ref{sec:integrity}, we provide integrity check by adding a redundant equation to each virtual batch. This leads to having $K+2$ linear equations for recovering $K+1$ unknowns. The extra equation can help us verify the solution of the first $K+1$ equation for the $K+1$ unknowns, in the last equation. If the solution is not consistent with the last equations, this means one of the GPU cores may not function properly or their data is modified by an attacker. So any single faulty computation or multiple non-colluding faulty computations can be detected. The forenamed system of linear equations is described below. 
\begin{equation}\label{eq:gamma_lin2}
\triangledown \mathbf{W}_{l} = \sum_{j=1}^{K+1}  \gamma_{j} \text{Eq}_{j}, \qquad \text{Eq}_{j} = \left\langle \sum_{i=1}^K \alpha_{j,i}~ \mathbf \delta^{(i)}_{l}~,~ \sum_{i=1}^K (\beta_{j,i}~ \mathbf x^{(i)}_{l}) + \beta_{j,(K+1)} ~{\mathbf r} \right\rangle~\quad~j=1,\dots K+2
\end{equation}

In order to avoid floating point arithmetic round off errors affecting our judgment on error detection, we define a threshold on the amount of data mismatch our system can tolerate. This threshold should be larger than the system precision because we do not want computation round off to be flagged as error. In a scenario where an adversary adds a perturbation to modify the result, If the amount of this perturbation is less than the system precision, it doesn't affect the convergence and hence we can discard it.
