# Supplementary material for: Privacy and Integrity Preserving Training Using Trusted Hardware
Source: arXiv:2105.00334 source file (2021-05-01)
Supplement: Supplementary file 2 [file Appendix6.tex]

\section{Slalom}

Among those approaches, \cite{tramer2018slalom} introduced Slalom an inference framework that uses TEEs to protect data privacy and integrity. Slalom uses the Intel SGX enclave to blind input data $\mathbf x$ from a client with an additive stream cipher noise $\mathbf r$. The blinded data $(\mathbf x +\mathbf r)$ is then sent to an untrusted GPU where linear operations are performed. The computed data  $\mathbf W \cdot (\mathbf x +\mathbf r)$ is then returned to the enclave which can decode the correct computational output $\mathbf W \cdot \mathbf x$ by subtracting the precomputed $\mathbf W \cdot \mathbf r$. Here $\mathbf W$ is the model parameter matrix.
Securely storing multiple instances of $\mathbf r$'s and their corresponding $\mathbf W \cdot \mathbf r$'s within the enclave memory, occupies a substantial amount of memory for large DNNs. On the other hand, storing an encrypted version of these values outside the enclave memory, leads to significant encryption and decryption costs, as these values are needed after each linear operation. In addition to that, Slalom cannot be used for training, since it precomputes $\mathbf W \cdot \mathbf r$. Precomputing the blinding factors is not feasible during training since the model parameters $\mathbf W$ are updated after processing every batch. Computing $\mathbf{W} \cdot \mathbf{r}$ inside the SGX after every batch also defeats the purpose of offloading the linear computations to GPU. Moreover, Slalom works on quantized models which needs a meticulous quantization algorithm not to affect the accuracy of training. Hence, the idea cannot be used in training as it is. Our idea addressed all the issues that Slalom paper introduced as its challenges for training.
