# Supplementary material for: Privacy and Integrity Preserving Training Using Trusted Hardware
Source: arXiv:2105.00334 source file (2021-05-01)
Supplement: Supplementary file 3 [file Appendix7.tex]

\section{GPU Comparison and Scalability}
Table~\ref{tab:GPUCMP} shows the performance of a baseline that uses GPU to perform the entire training. Clearly users of this baseline cannot protect their data. However, using a GPU for training large DNNs can give us 120X speedup relative to baseline fully implemented on SGX.  DarKnight bridges  this gap by more than 10X while protecting data privacy. Hence, there is no free lunch to obtain privacy, but our goal is to provide the best performance when privacy is not optional, as is the case in many operational settings such as medical imaging. 

\begin{table}[htb]
\caption{Speedup in GPU relative to SGX in VGG16 Training on ImageNet. The baseline is implemented fully on Intel SGX}
\label{tab:GPUCMP}
\centering
\resizebox{0.8\columnwidth}{!}{%
\begin{tabular}{c cccc}
\hline

Operations & Linear Ops  & Maxpool Time & Relu Time & Total \\ \hline
Forward Pass    & 126.85  & 11.86  & 119.60 & 119.03         \\
Backward Propagation  & 149.13  & 5.47 & 6.59 &  124.56 \\
\hline
\centering
\end{tabular}
}
\end{table}

As we showed in our earlier analysis DarKnight tilts the computational balance from linear operations to non-linear operations running on SGX. Hence, the overall execution time is determined by SGX performance. But this tradeoff is not a fundamental bottleneck to scalability. With the shift towards server disaggregation~\cite{lim2009disaggregated,guleria2019quadd} in the cloud it is possible to separate GPU pool from CPU pool and increase the number of concurrent SGX enclaves that can concurrently feed a GPU. Furthermore, DarKnight can be seamlessly adapted to a distributed training platform that uses data parallelism across GPUs, since inputs sent to different GPUs can be concurrently blinded using a dedicated set of SGX enclaves that feed these GPUs. Hence, we believe DarKnight has cost-effective scalability characteristics when privacy is an important consideration in training.
