# Supplementary material for: Privacy and Integrity Preserving Training Using Trusted Hardware
Source: arXiv:2105.00334 source file (2021-05-01)
Supplement: Supplementary file 4 [file Appendix5.tex]

\section{Adversarial Attacks}:
Please note that data poising attacks and model poisoning attacks are out of the scope of this work. \\
In this section we examine two scenarios. In the first scenario, the invader bombards the model with images to find out the encoding parameters. in this case since the parameters such as Matrix $\mathbf A$ and random noise $\mathbf r$ are generated for each batch and and never reused during the execution time, even if an adversary can extract them, there will not be useful. \\

In this scneraio
